# Supplementary material for: Leveraging Medical Visual Question Answering with Supporting Facts
Source: arXiv:1905.12008 source file (2019-05-28)
Supplement: Supplementary file 1 [file appendix.tex]

\section{Exemplary results}
\label{sec:exemplary_results}

\tk{In here we will show some correct and incorrect samples (images, questions, ground truth answers that predicted answers)}

image id: synpic50359	
question: ['what', 'organ', 'system', 'is', 'pictured', 'here']
target: heart and great vessels \# lung, mediastinum, pleura
prediction: spine and contents
